# Supplementary material for: Bayesian truncation errors in chiral effective field theory: nucleon-nucleon observables
Source: arXiv:1704.03308 ancillary file (2017-08-25)
Supplement: Supplementary file 1 [file Supplemental_Material.pdf]

# Supplemental material for Bayesian truncation errors in chiral effective field theory: nucleon-nucleon observables

J. A. Melendez,<sup>\*</sup> S. Wesolowski,<sup>†</sup> and R. J. Furnstahl<sup>‡</sup>  
*Department of Physics, The Ohio State University, Columbus, OH 43210, USA*  
(Dated: August 24, 2017)

Additional figures documenting the conclusions in this paper.

---

<sup>\*</sup> melendez.27@osu.edu  
<sup>†</sup> wesolowski.14@osu.edu  
<sup>‡</sup> furnstahl.1@osu.edu

# I. SUPPLEMENTAL MATERIAL

Here we collect additional informative figures to supplement those in the text.

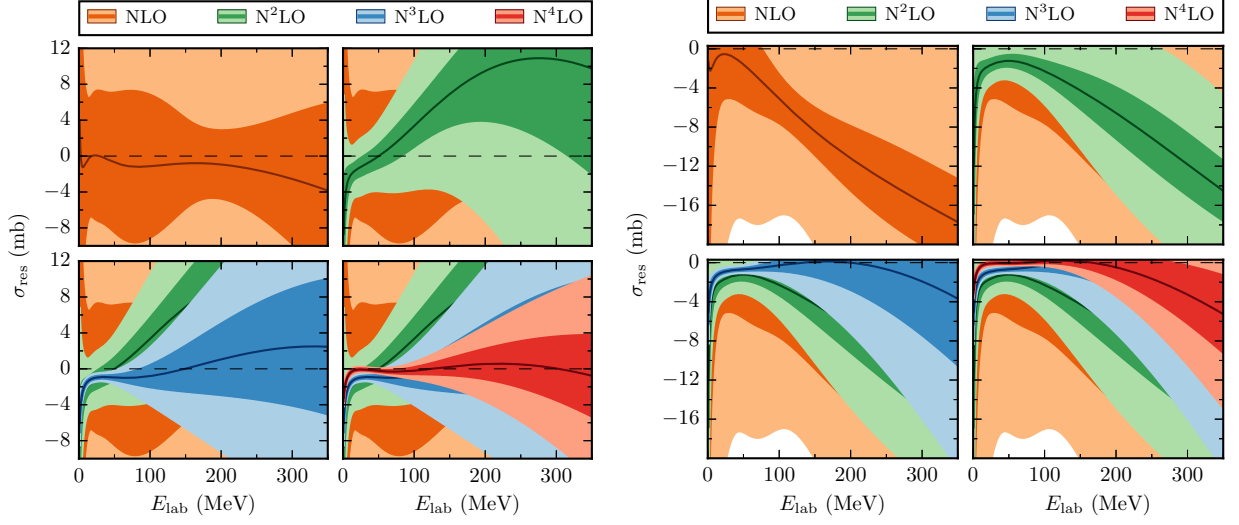

FIG. 1. Residuals at each order for the total  $np$  cross section with DoB intervals calculated using prior set  $C_{0.25-10}$  and  $\Lambda_b = 600$  MeV. Left:  $R = 0.8$  fm, and right:  $R = 1.0$  fm.

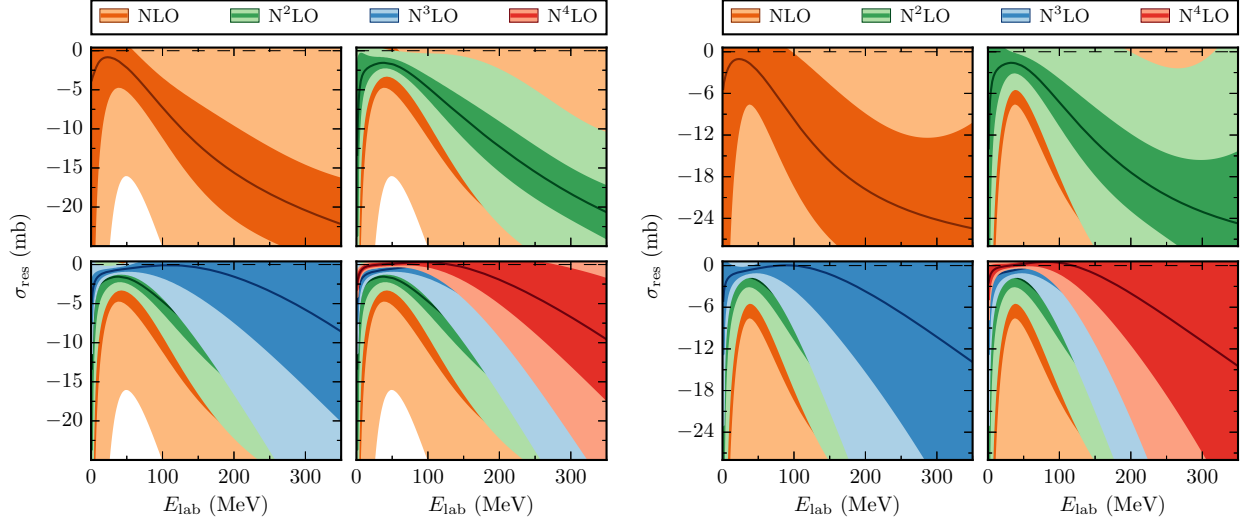

FIG. 2. Residuals at each order for the total  $np$  cross section with DoB intervals calculated using prior set  $C_{0.25-10}$ . Left:  $R = 1.1$  fm with  $\Lambda_b = 500$  MeV, and right:  $R = 1.2$  fm with  $\Lambda_b = 400$  MeV.

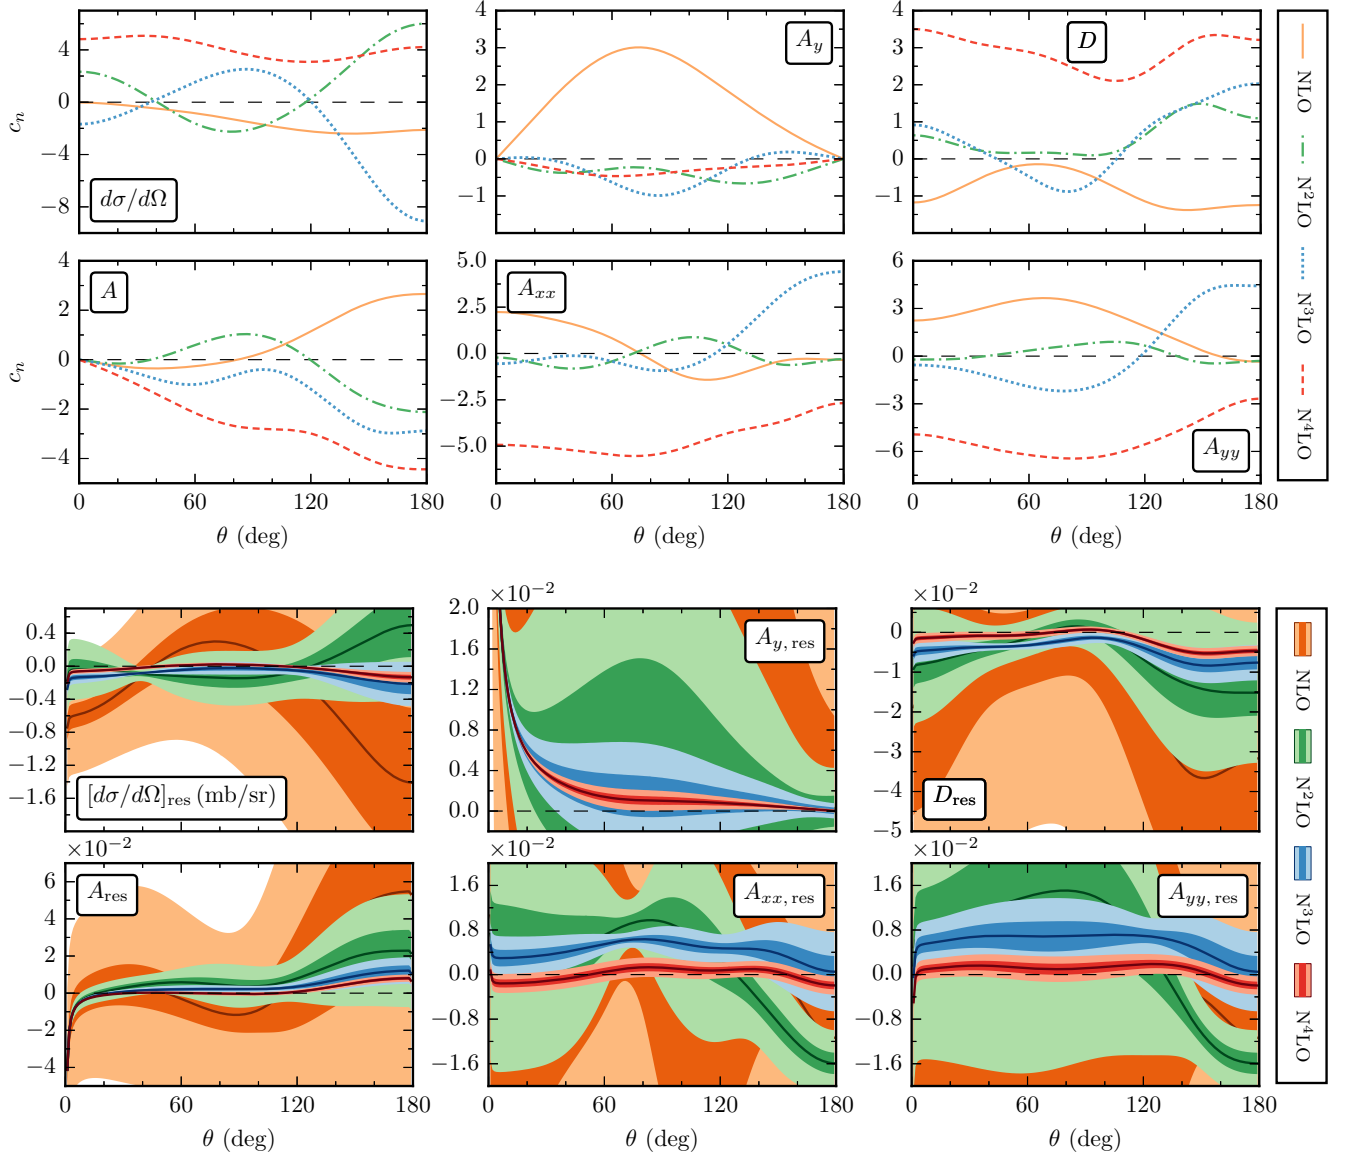

FIG. 3. Top: Observable coefficients for  $E_{\text{lab}} = 50$  MeV with  $X_{\text{ref}} = X_0$  for the differential cross section and  $X_{\text{ref}} = 1$  for all other spin observables. Bottom: Residuals with error bands generated using prior set  $C_{0.25-10}$ .

TABLE I. Observable coefficients  $b_n$  for the  $np$  total cross section in units of  $\text{MeV}^{-n}$ . Lab energy  $E_{\text{lab}}$  and relative momentum  $p_{\text{rel}}$  are in units of MeV.

| $E_{\text{lab}}$ | $p_{\text{rel}}$ | $b_2 \times 10^6$ | $b_3 \times 10^9$ | $b_4 \times 10^{12}$ | $b_5 \times 10^{15}$ |
|------------------|------------------|-------------------|-------------------|----------------------|----------------------|
| 50               | 153              | -4.24             | 0.763             | -1.82                | 50.2                 |
| 96               | 212              | -2.63             | 4.14              | -4.86                | 14.7                 |
| 143              | 259              | -0.975            | 5.77              | -2.18                | 2.53                 |
| 200              | 307              | 0.300             | 6.66              | 2.07                 | -5.70                |
| 300              | 375              | 1.26              | 6.24              | 8.64                 | -11.4                |

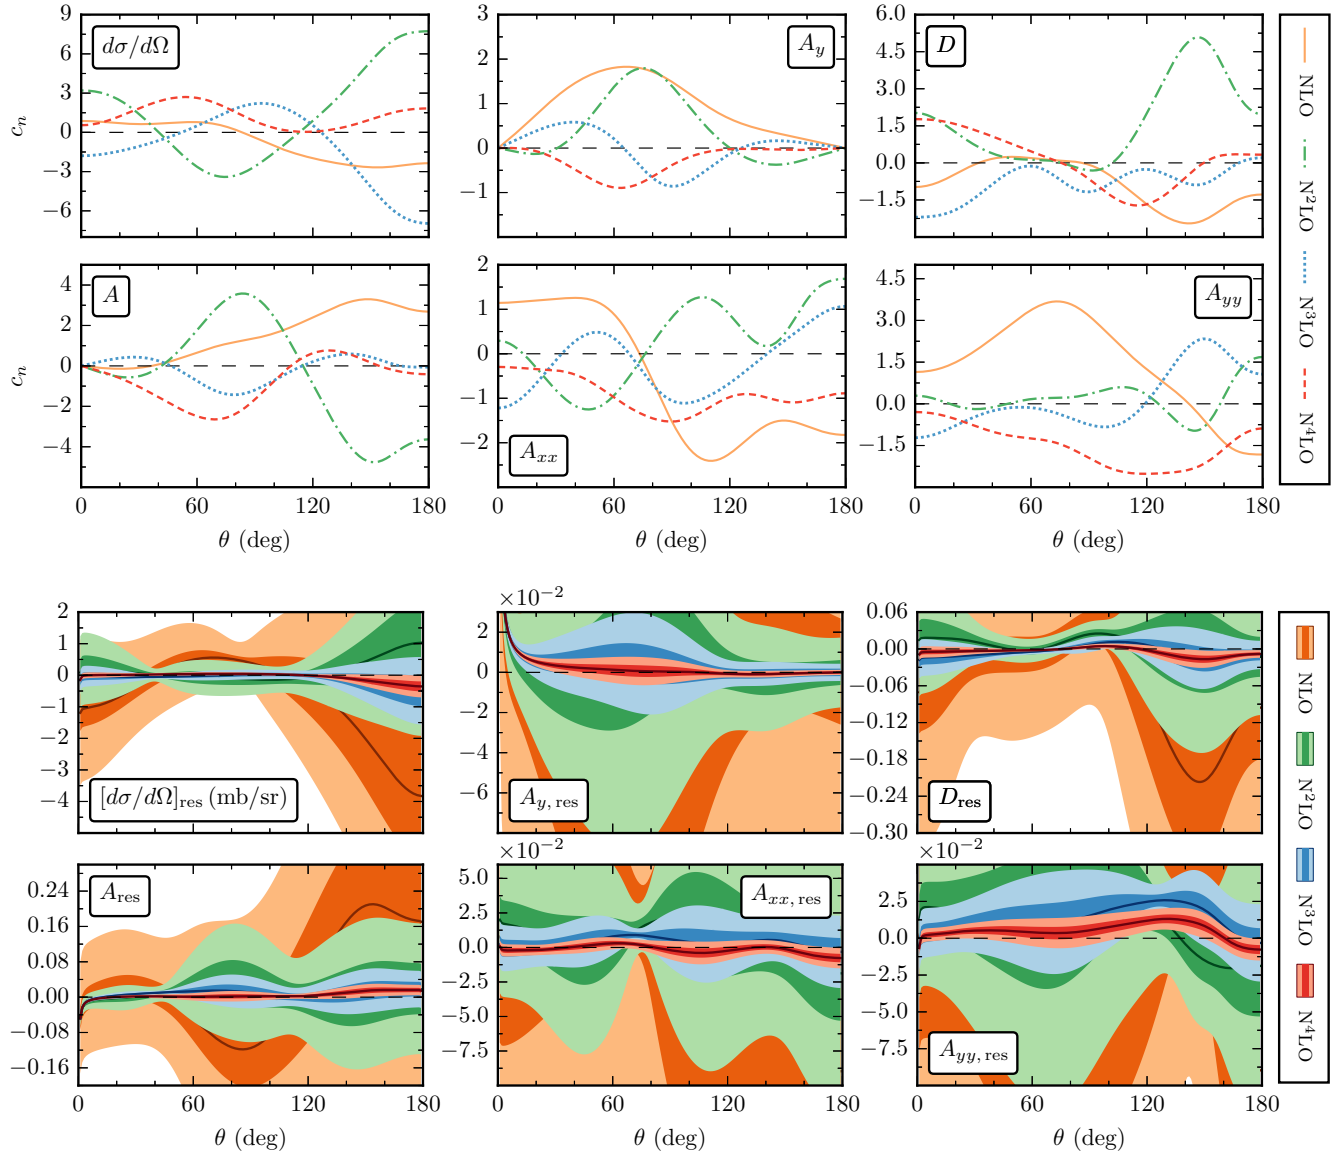

FIG. 4. Same as Fig. 3, but with  $E_{\text{lab}} = 96$  MeV.

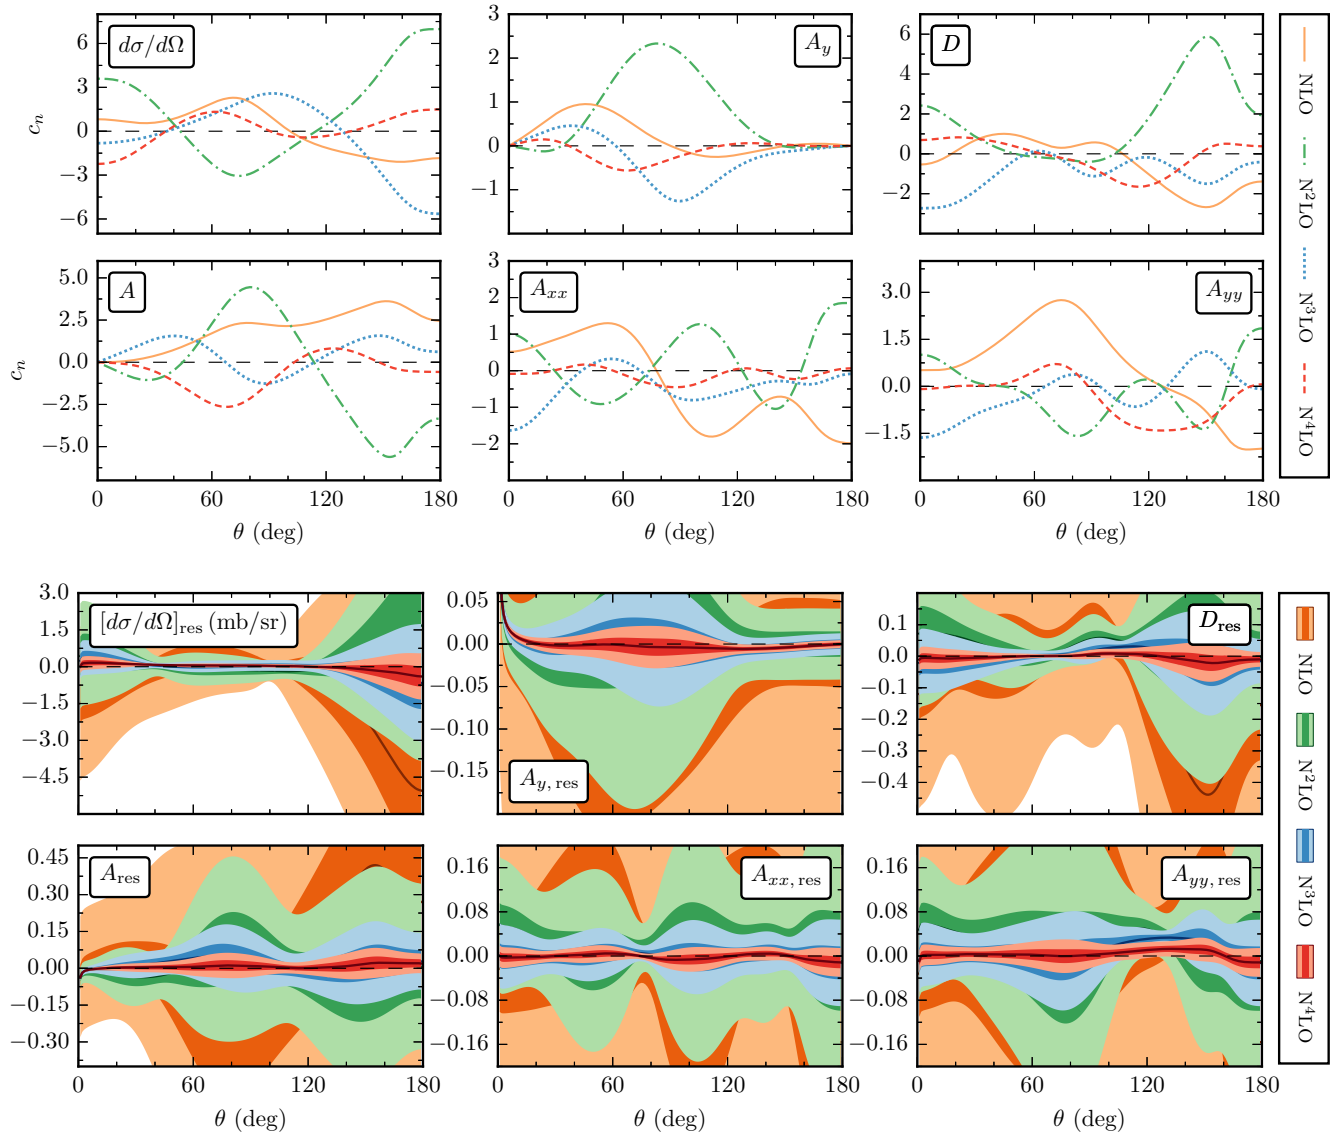

FIG. 5. Same as Fig. 3, but with  $E_{\text{lab}} = 143 \text{ MeV}$ .

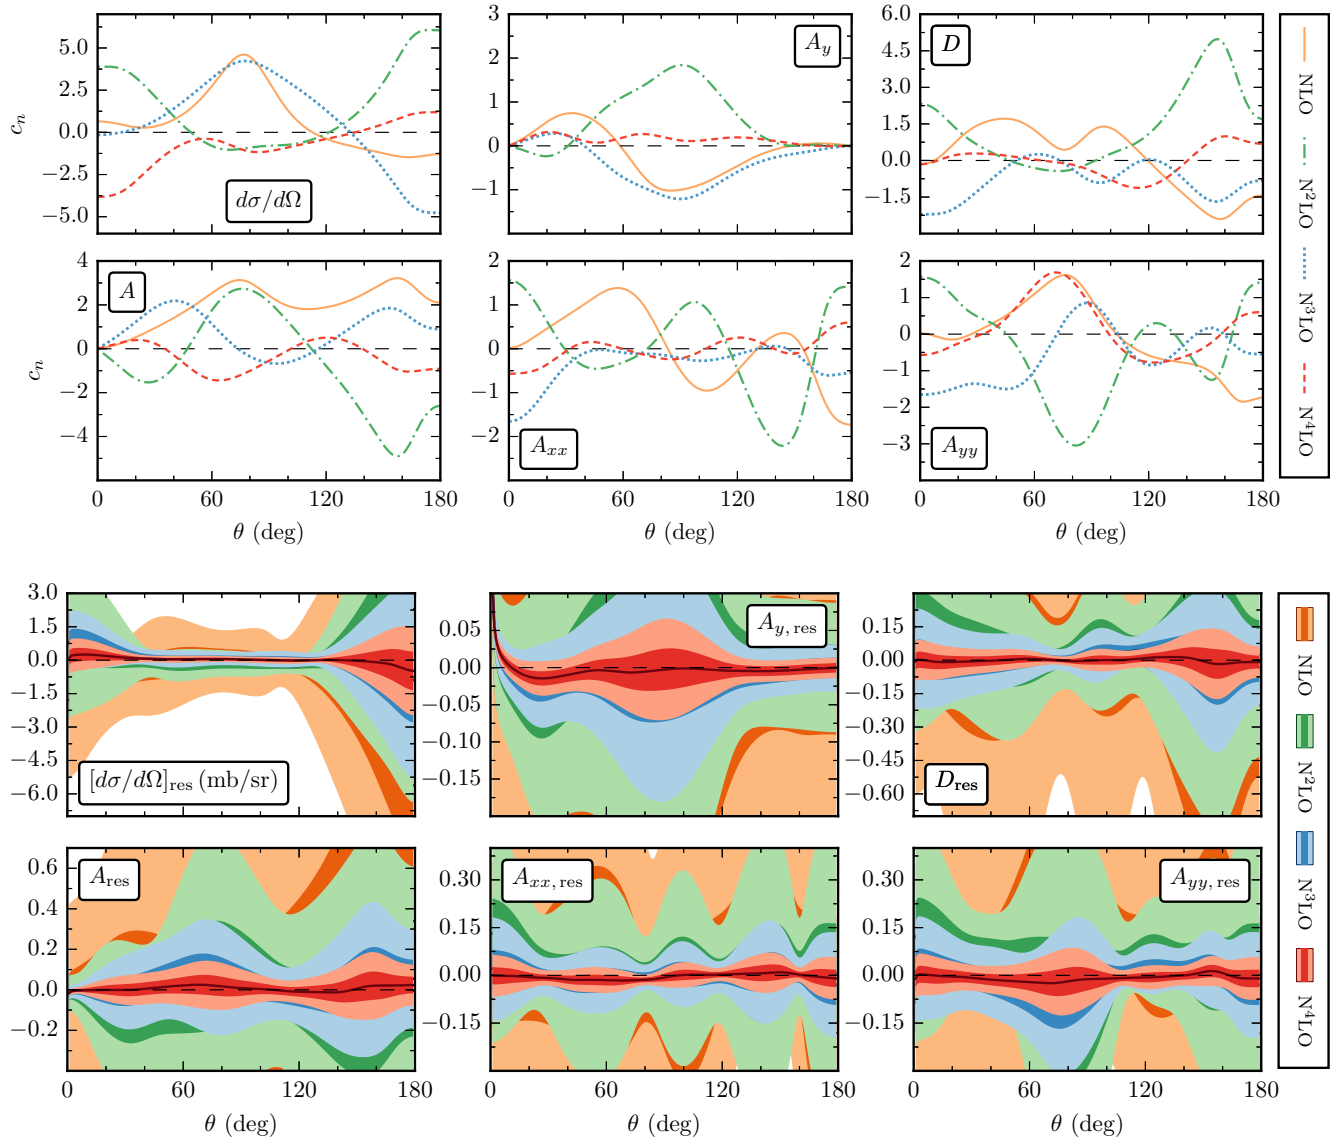

FIG. 6. Same as Fig. 3, but with  $E_{\text{lab}} = 200$  MeV.

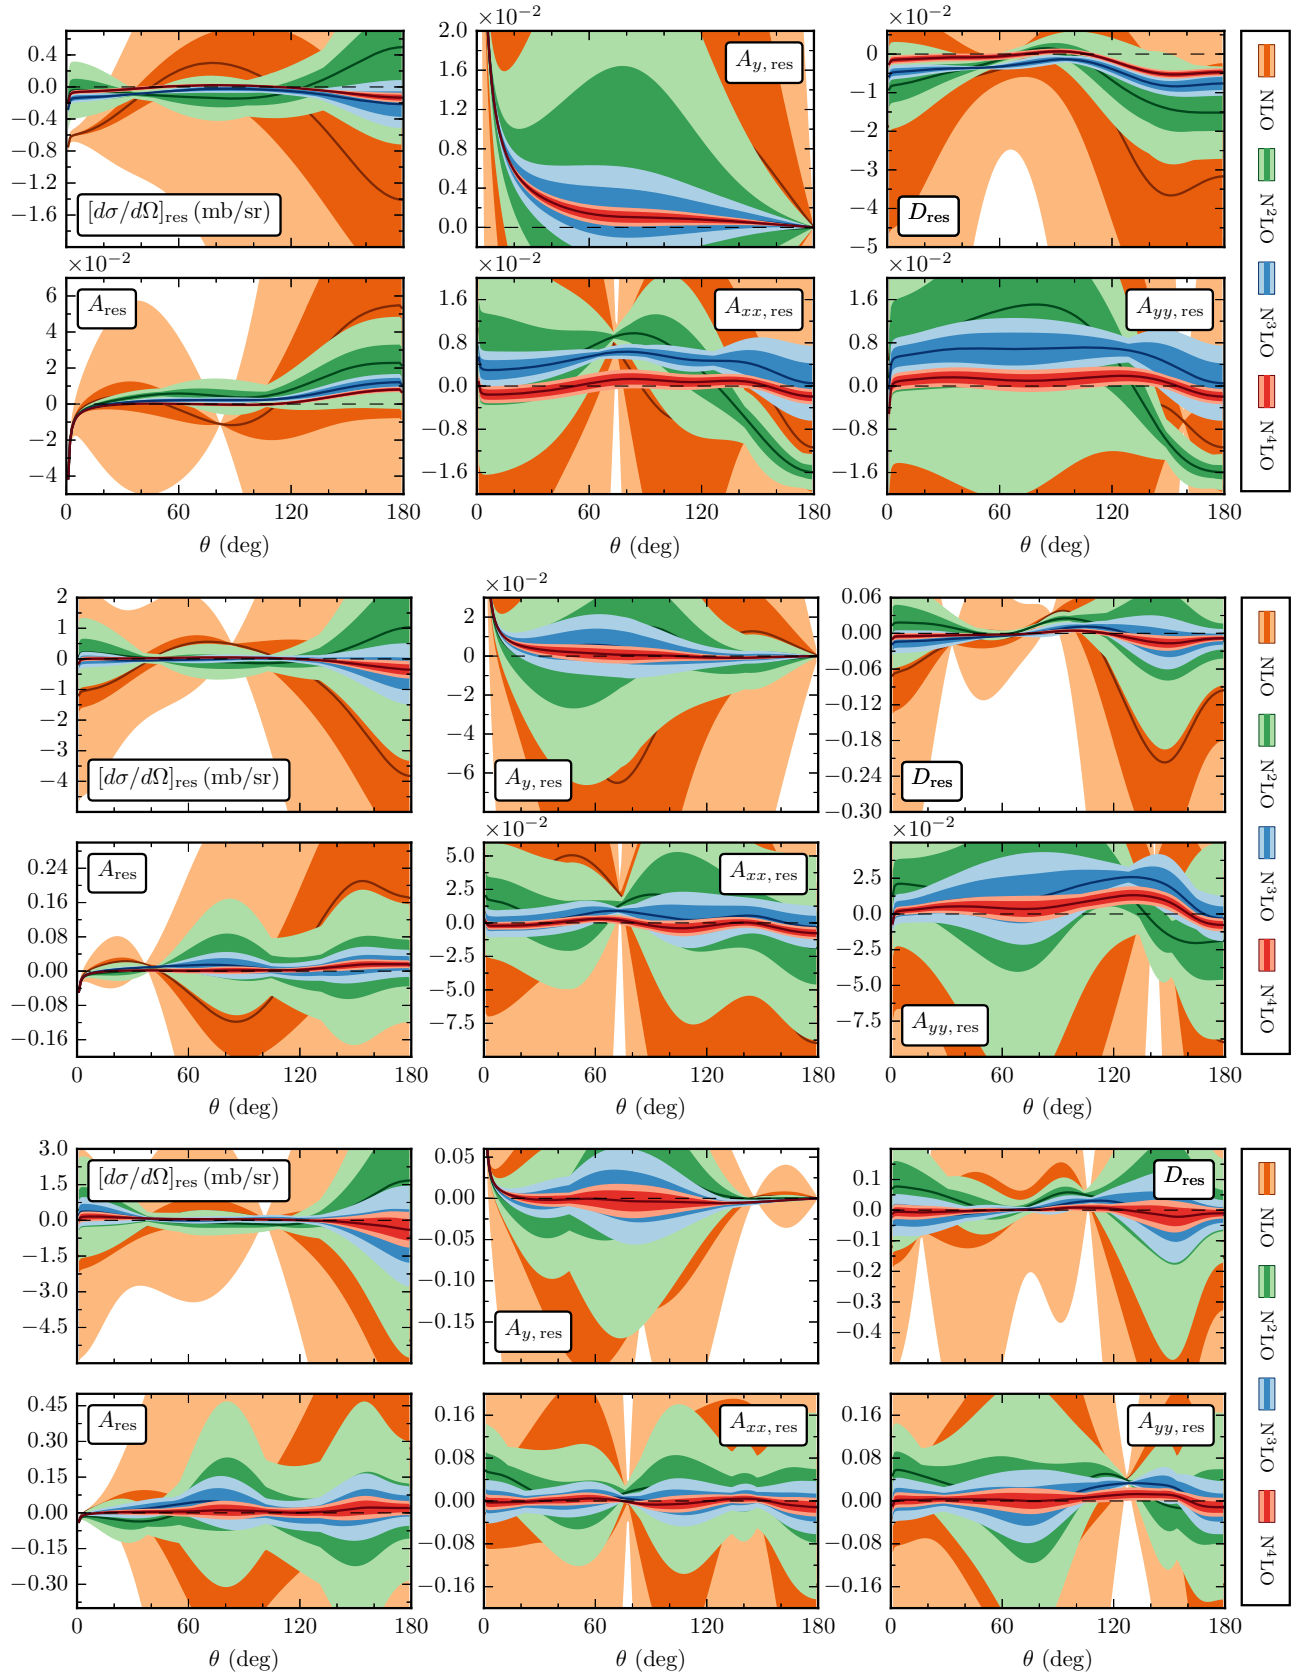

FIG. 7. Residuals computed using the  $R = 0.9$  fm EKM potential with DoBs generated using  $A_\epsilon^{(1)}$ . Top, middle, and bottom plot use  $E_{\text{lab}} = 50, 96, 143$  MeV, respectively.

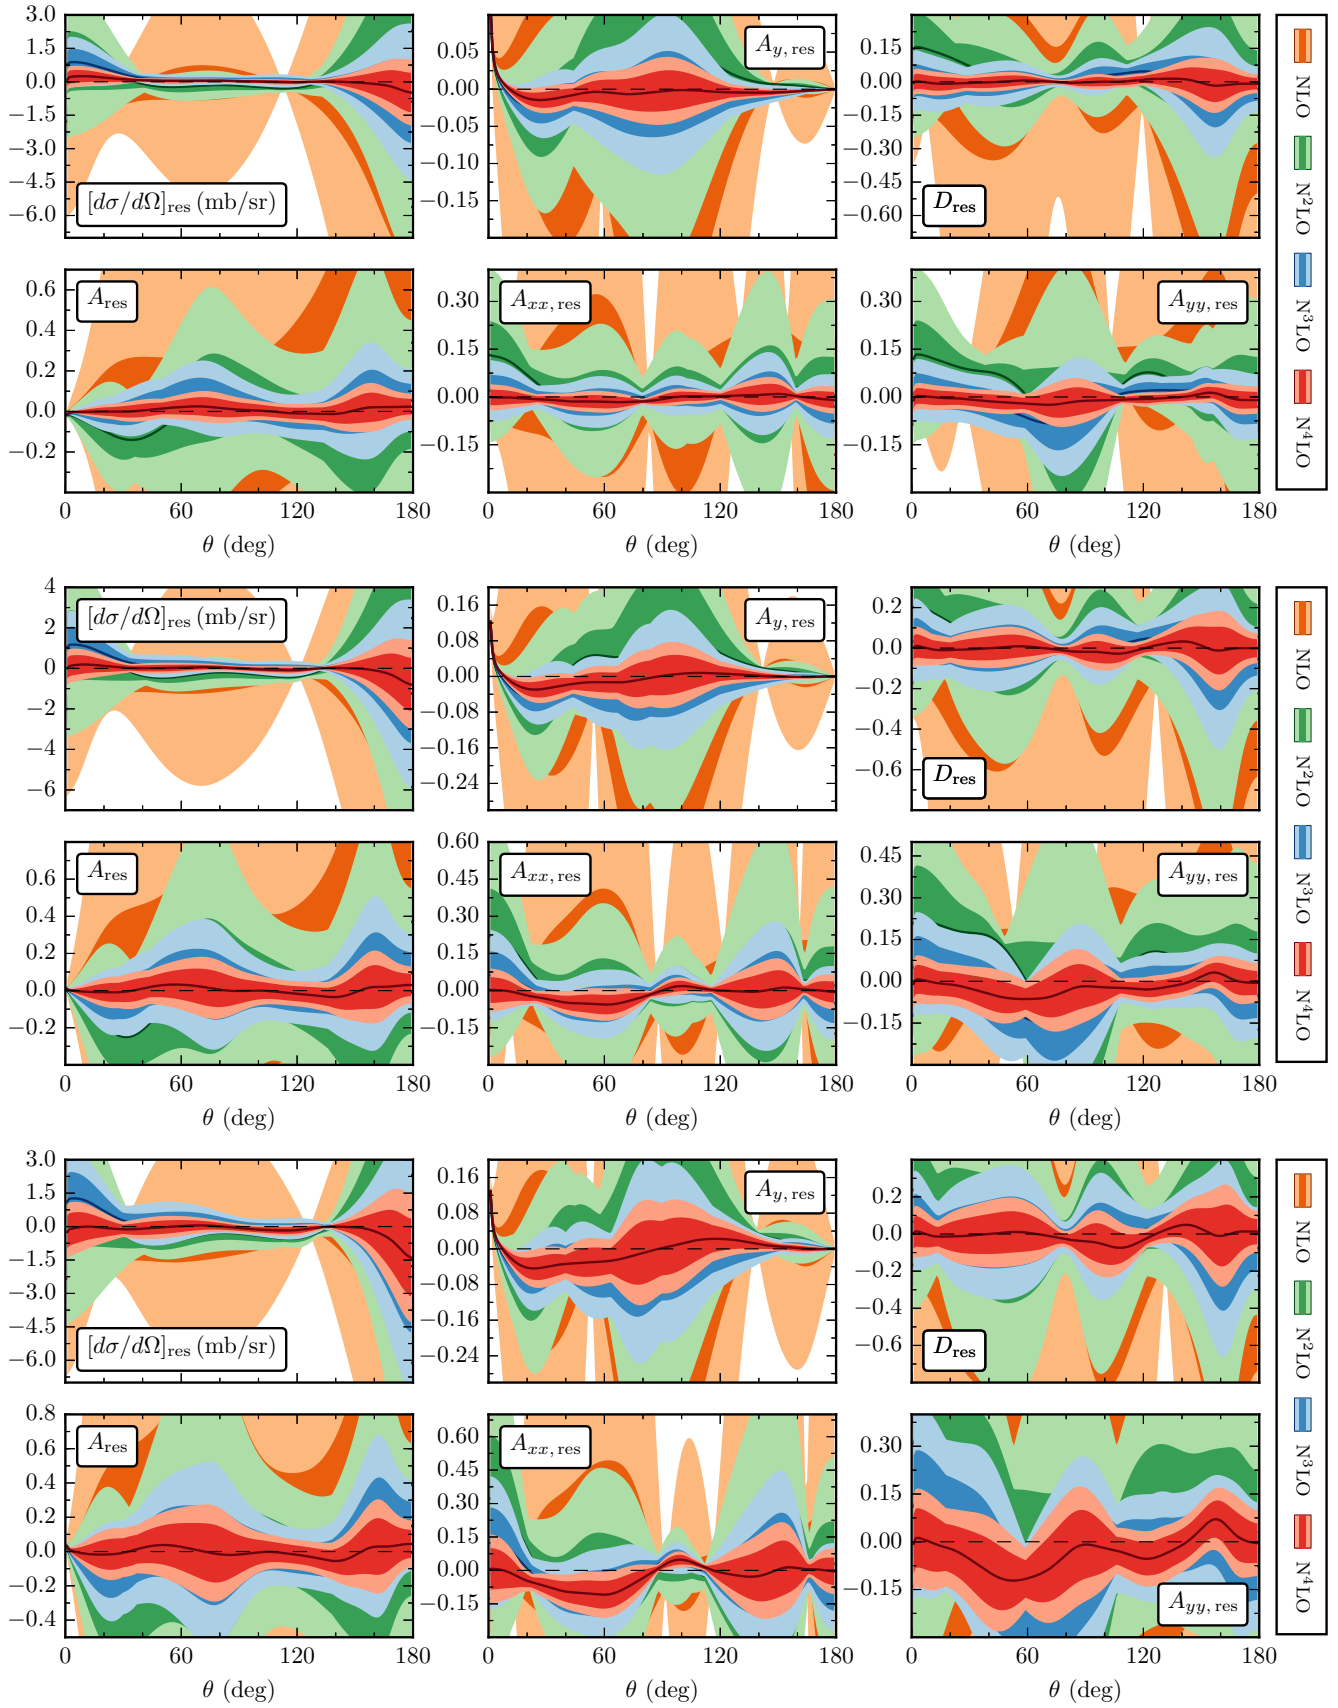

FIG. 8. Same as Fig. 7, but the top, middle, and bottom plot use  $E_{\text{lab}} = 200, 250, 300$  MeV, respectively.

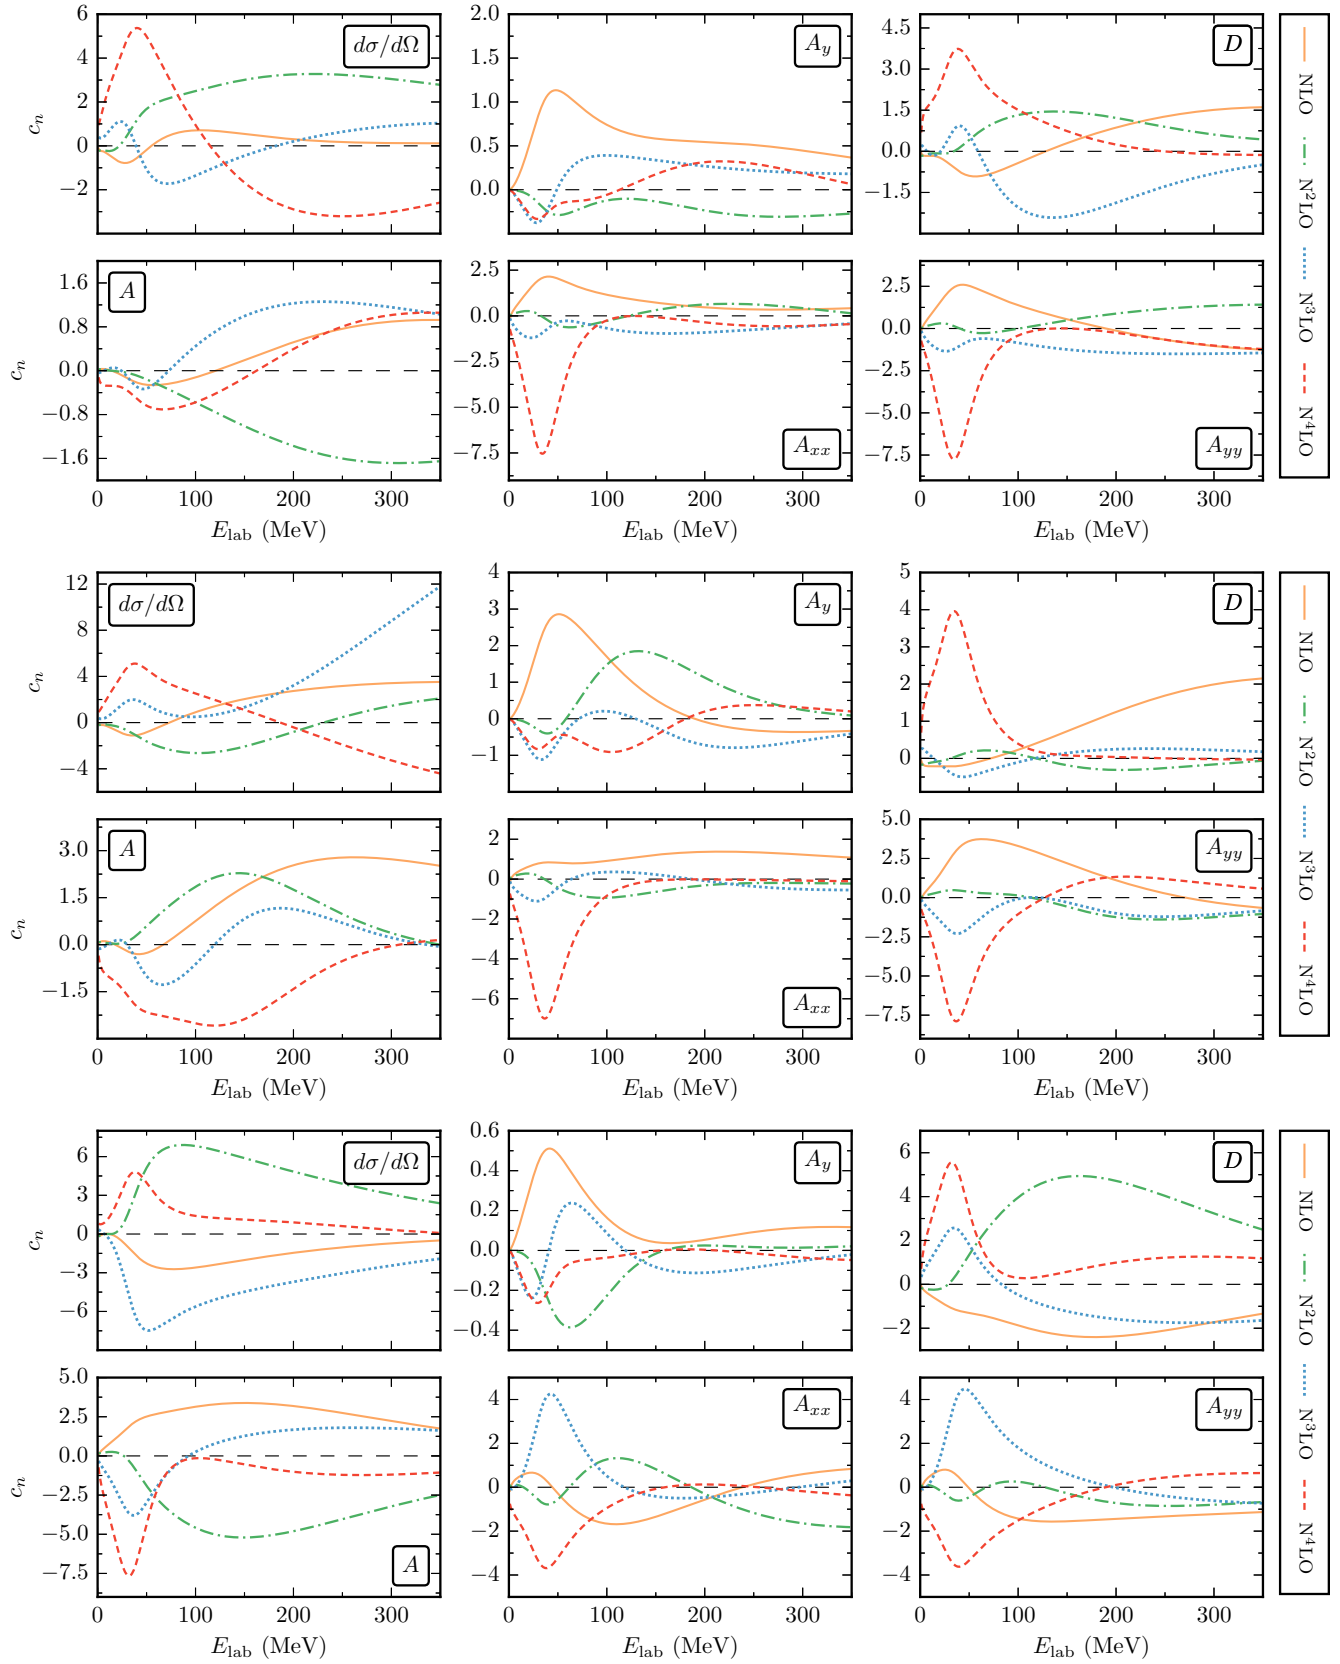

FIG. 9. Coefficients for various angle-dependent observables vs  $E_{\text{lab}}$  using the  $R = 0.9\text{ fm}$  EKM potential. Top, center, and bottom plots use  $\theta = 20^\circ, 60^\circ, 160^\circ$ , respectively.

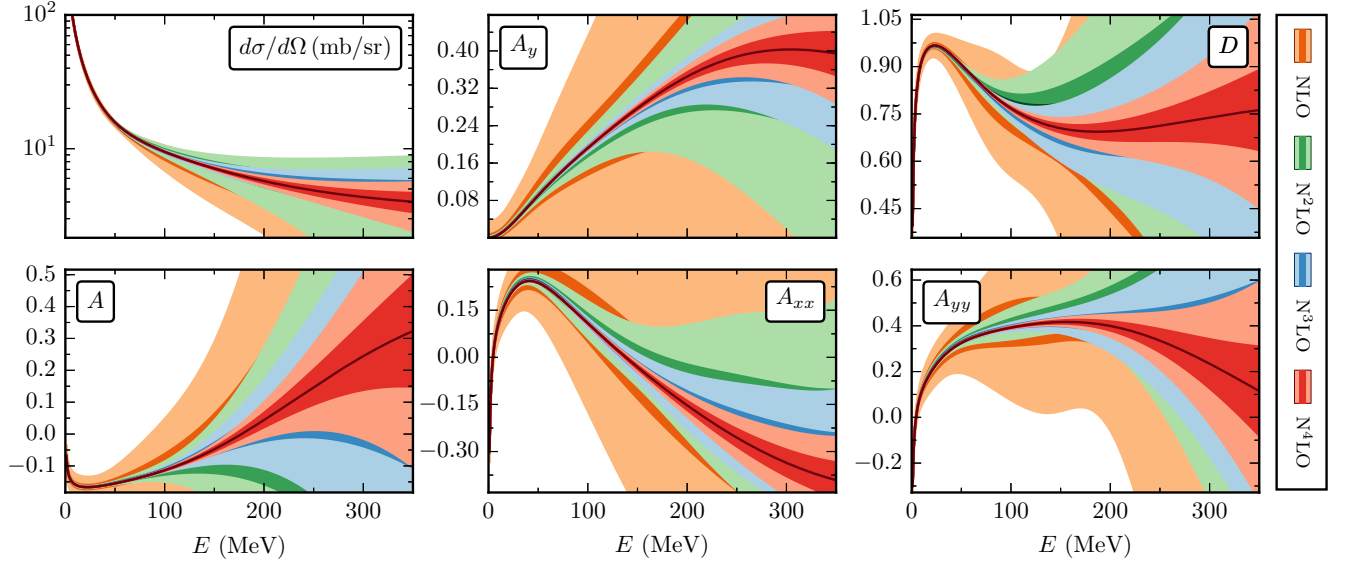

FIG. 10. Observables at  $\theta = 20^\circ$  generated using the  $R = 0.9$  fm EKM potential with error bands from prior set  $C_{0.25-10}$ .

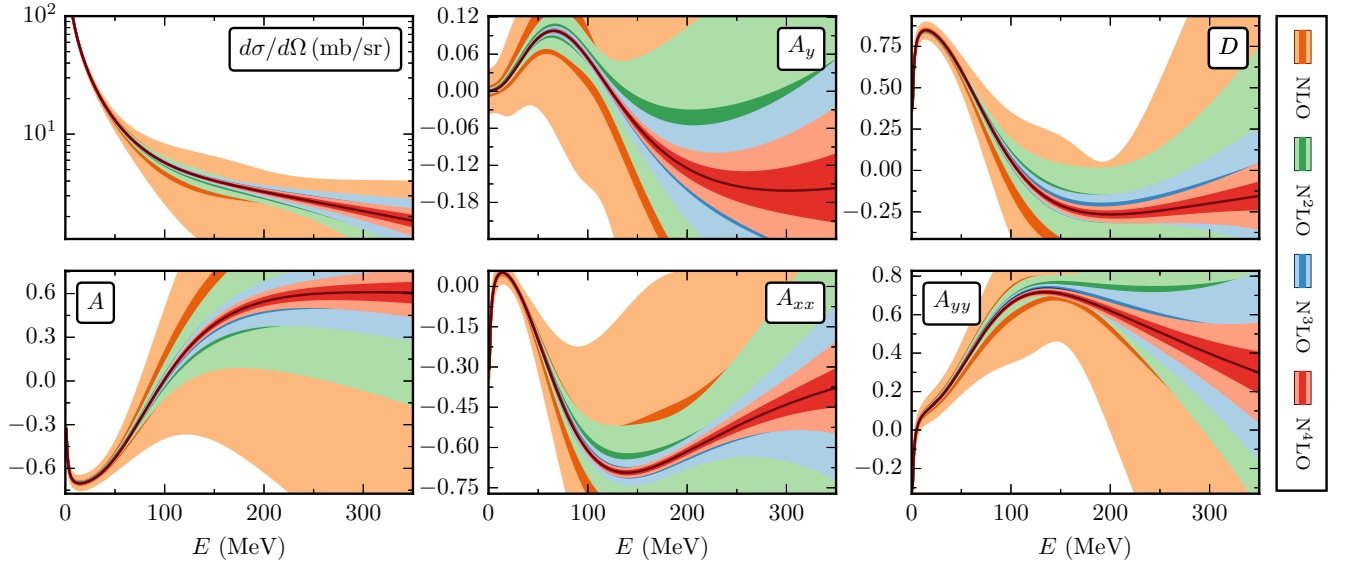

FIG. 11. Observables at  $\theta = 120^\circ$  generated using the  $R = 0.9$  fm EKM potential with error bands from prior set  $C_{0.25-10}$ .

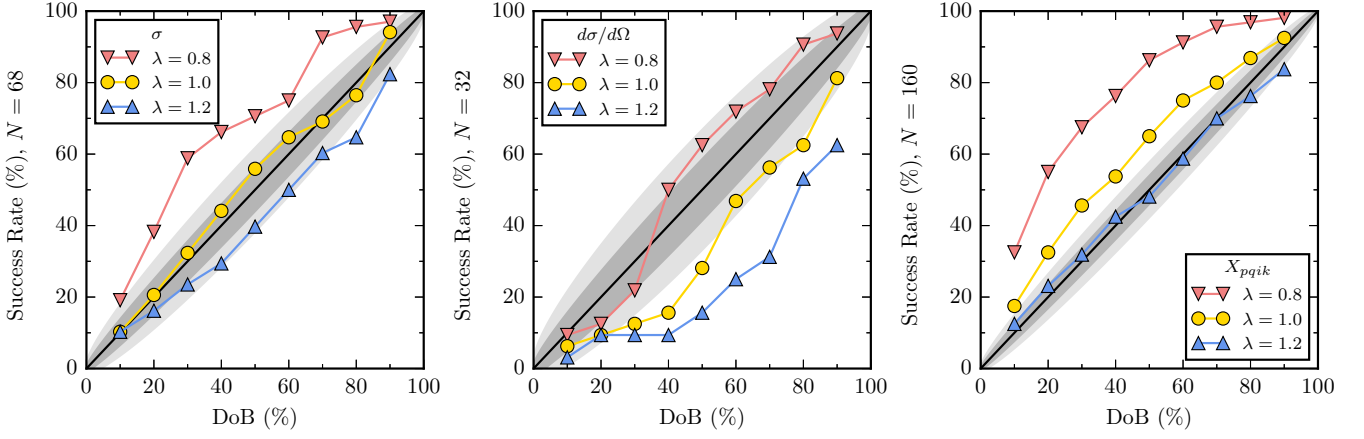

FIG. 12. Consistency plots comparing the NLO–N<sup>4</sup>LO averaged error band success rate to NPWA data for  $R = 0.9$  fm and prior set  $C_{0.25-10}$ . The total cross section is evaluated at  $E_{\text{lab}} = 20, 40, \dots, 340$  MeV, while the rest are evaluated at  $E_{\text{lab}} = 96, 143, 200, 300$  MeV and  $\theta = 60^\circ, 120^\circ$ .

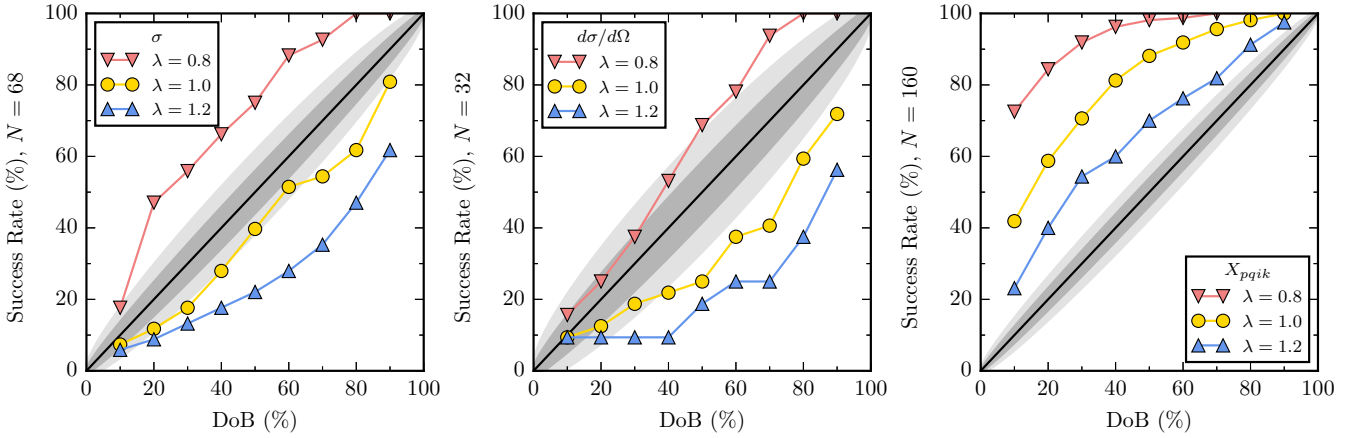

FIG. 13. Consistency plots as in Fig. 12, but with  $R = 1.2$  fm.

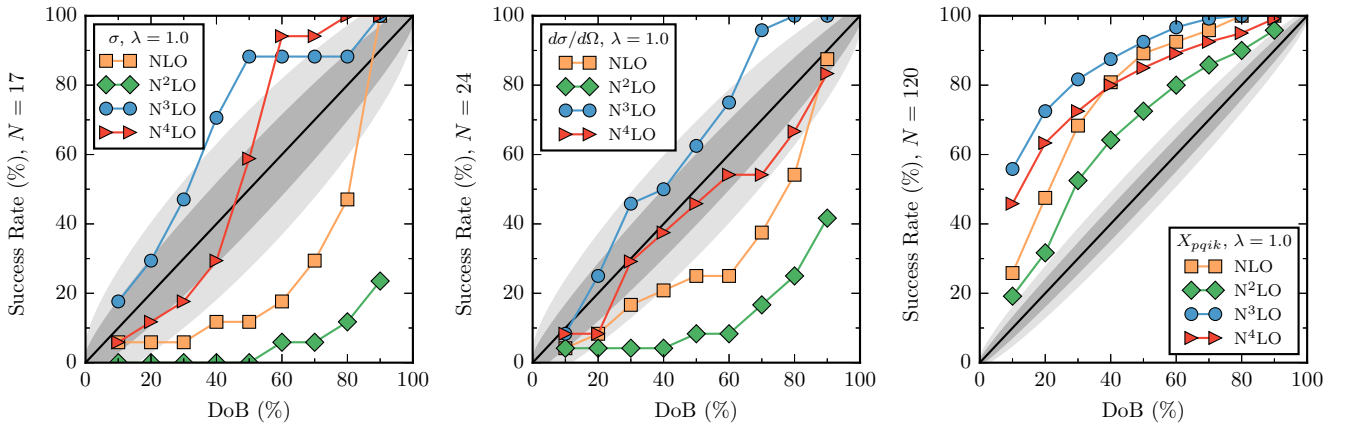

FIG. 14. Consistency plots comparing the order-by-order NLO–N<sup>4</sup>LO error band success rate to NPWA data for  $R = 1.2$  fm and prior set  $C_{0.25-10}$ . The total cross section is evaluated at  $E_{\text{lab}} = 20, 40, \dots, 340$  MeV, while the rest are evaluated at  $E_{\text{lab}} = 96, 143, 200, 300$  MeV and  $\theta = 40^\circ, 60^\circ, \dots, 140^\circ$ .

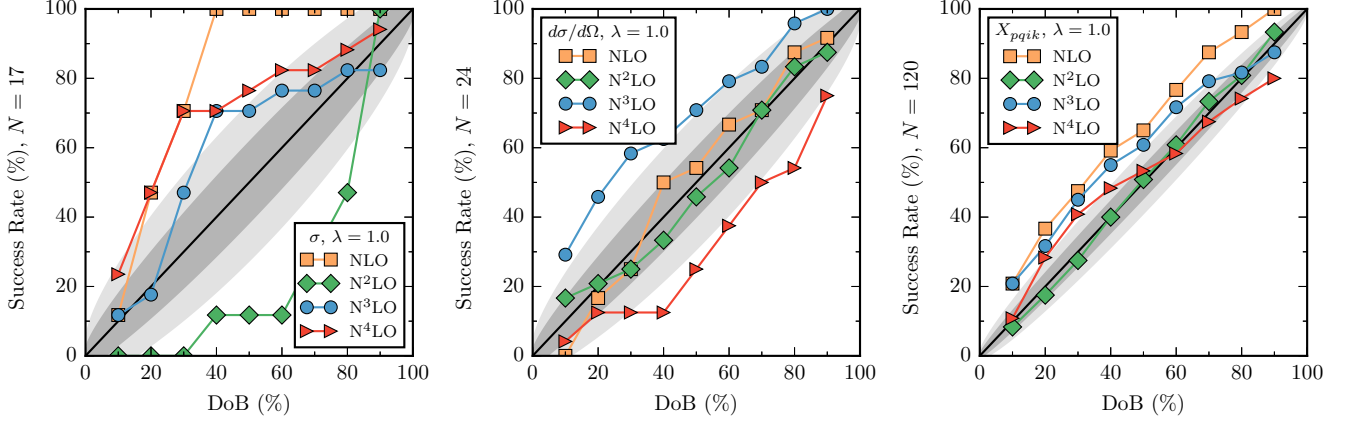FIG. 15. Same as Fig. 14 but with  $R = 0.8$  fm.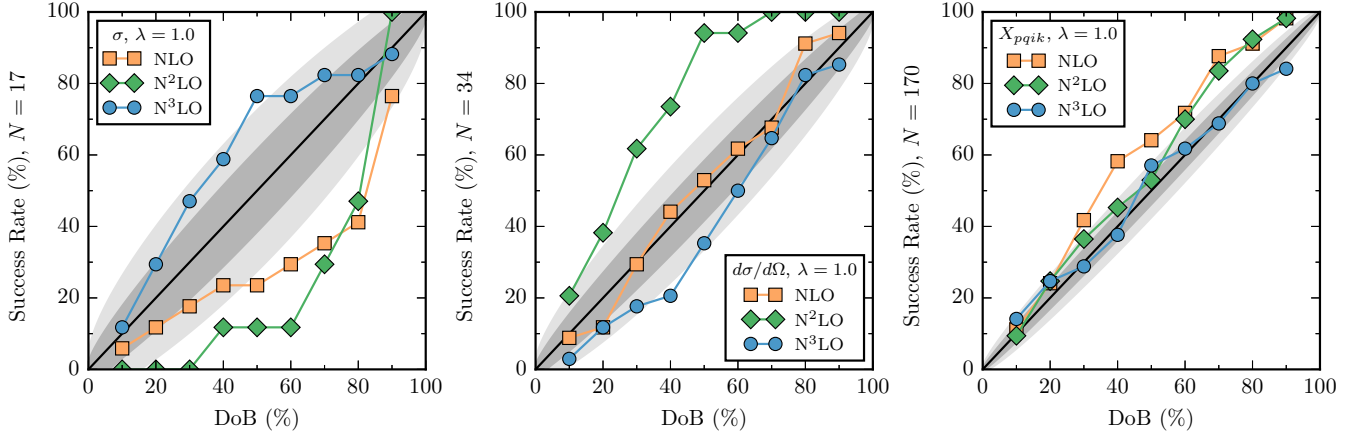FIG. 16. Consistency plots with the  $R = 0.8$  fm EKM potential showing order-by-order results for  $C_{0.25-10}^{(1)}$ . Here  $\theta = 60^\circ, 120^\circ$  and  $E_{\text{lab}} = 20, 40, \dots, 340$  MeV.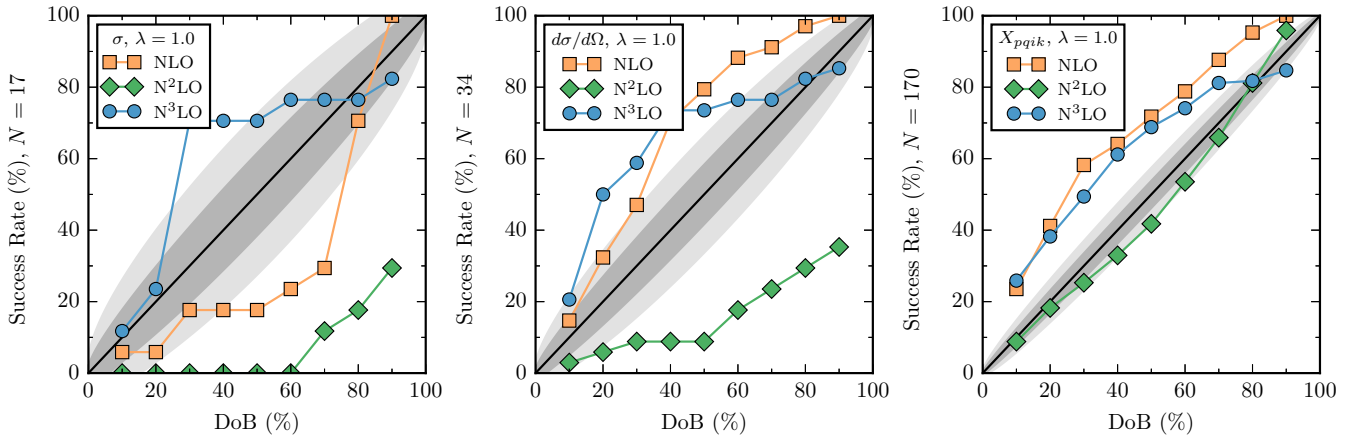FIG. 17. Consistency plots with the  $R = 1.0$  fm EKM potential showing order-by-order results for  $C_{0.25-10}^{(1)}$ . Here  $\theta = 60^\circ, 120^\circ$  and  $E_{\text{lab}} = 20, 40, \dots, 340$  MeV.

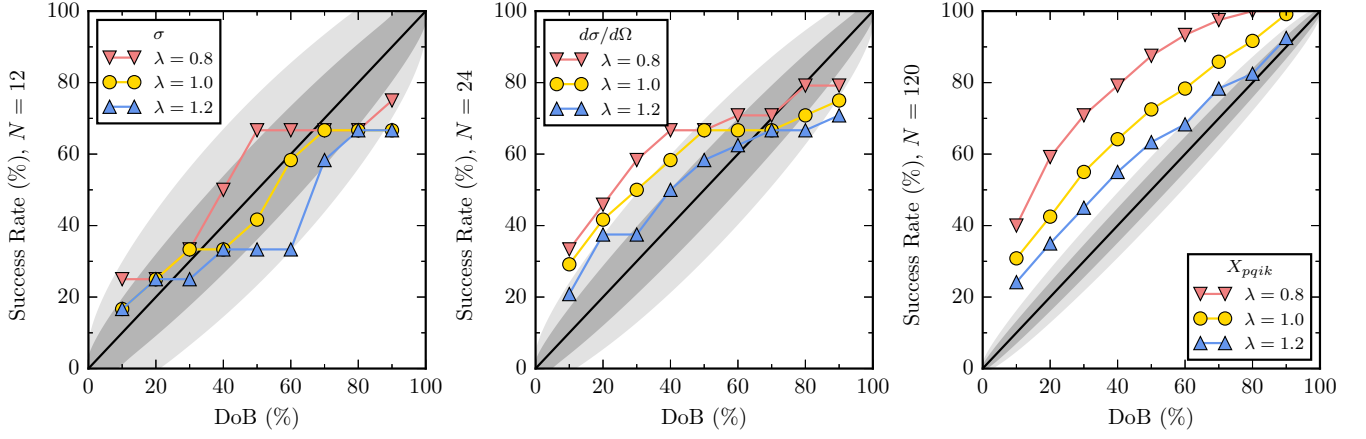

FIG. 18. Consistency plots using  $C_{0.25-10}^{(1)}$  averaged over NLO–N<sup>3</sup>LO results for various observable sets with  $R = 1.1$  fm. Observables are evaluated at  $E_{\text{lab}} = 96, 143, 200, 300$  MeV and at  $\theta = 60^\circ, 120^\circ$  if applicable.

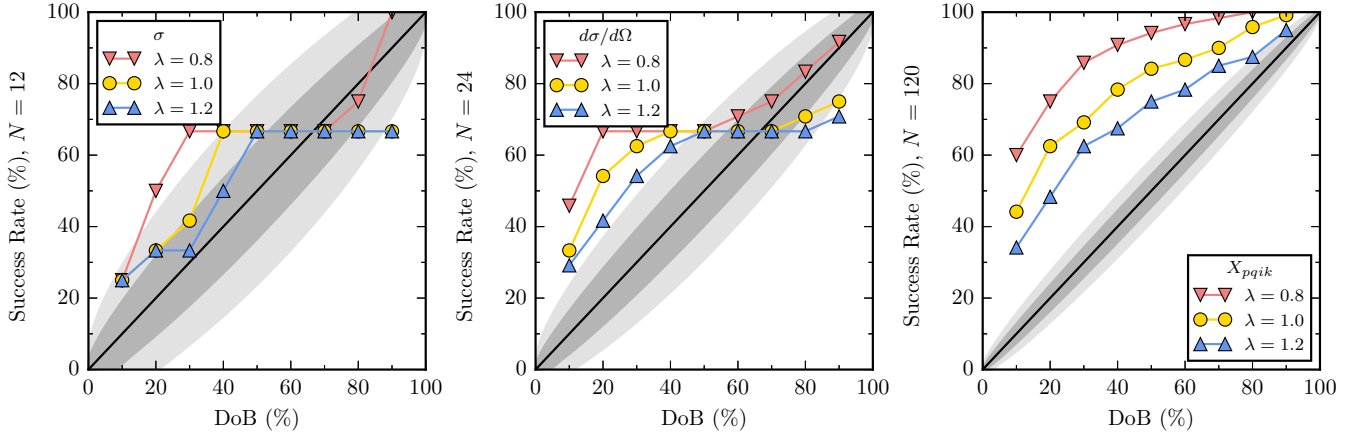

FIG. 19. Same as Fig. 18, but with  $R = 1.2$  fm.

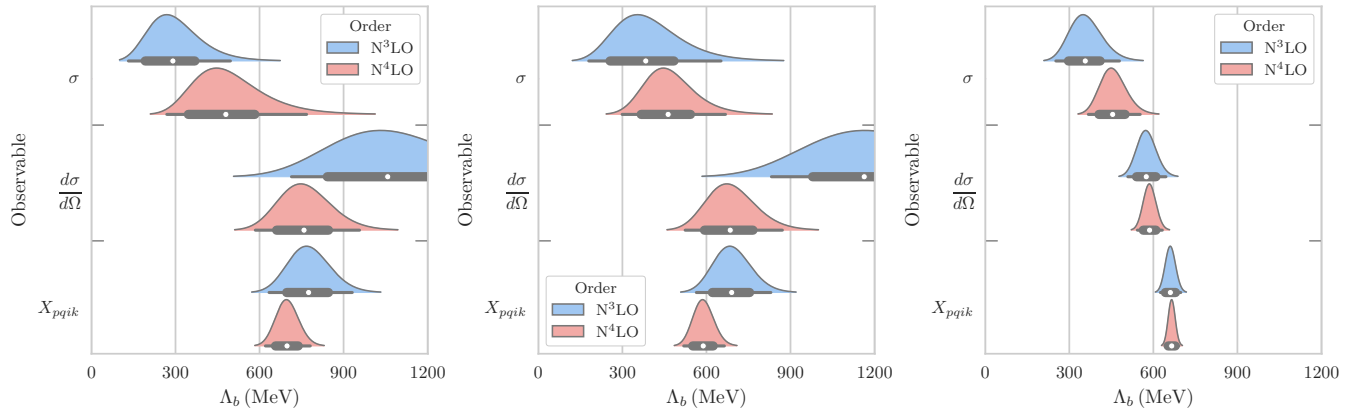

FIG. 20.  $\Lambda_b$  posterior plots generated using the  $R = 0.8$  fm EKM potential. Left, center, and right plots use  $E_{\text{lab}} = 96, 143, 200, 300$  MeV and  $\theta = 60^\circ, 120^\circ$ ;  $E_{\text{lab}} = 50, 96, 143, 200$  MeV and  $\theta = 60^\circ, 120^\circ$ ; and  $E_{\text{lab}} = 20, 40, \dots, 340$  MeV and  $\theta = 40^\circ, 60^\circ, \dots, 140^\circ$ , respectively.

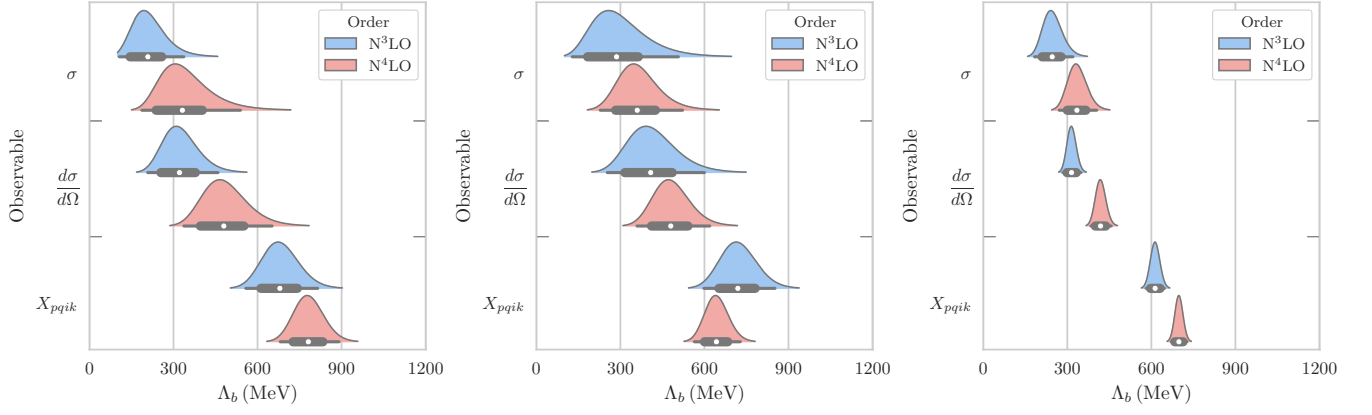

FIG. 21. Same as Fig. 20, but with the  $R = 1.0$  fm EKM potential.

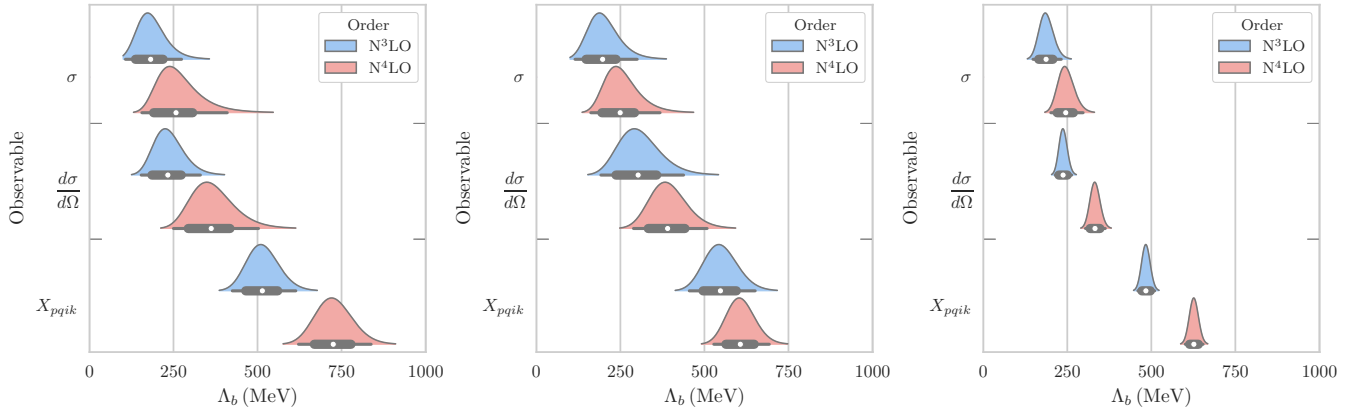

FIG. 22. Same as Fig. 20, but with the  $R = 1.1$  fm EKM potential.

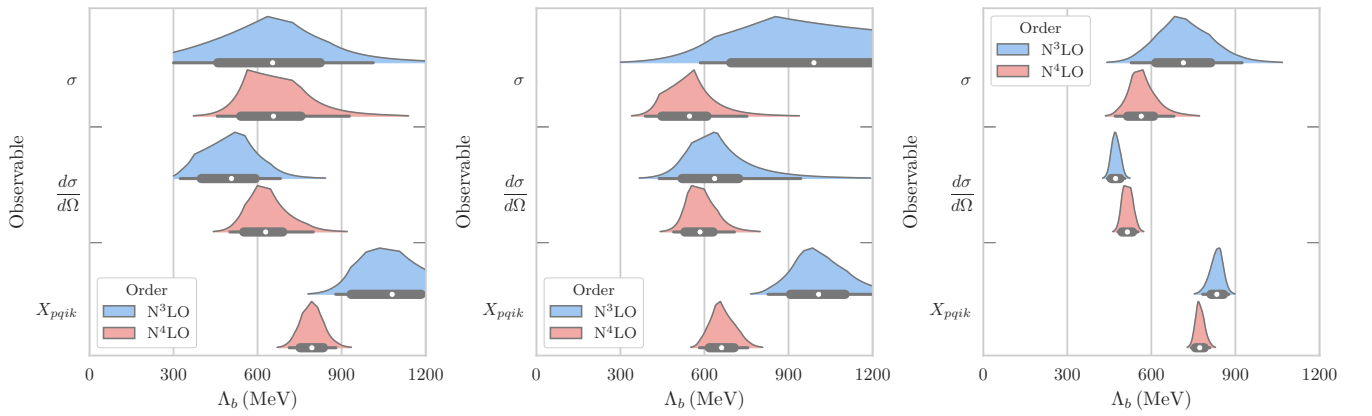

FIG. 23. Same as Fig. 20, but with the  $R = 0.9$  fm EKM potential and using set  $A_\epsilon$ .
